# Supplementary material for: A Comprehensive Survey of Deep Learning for Time Series Forecasting: Architectural Diversity and Open Challenges
Source: arXiv:2411.05793 source file (2025-05-01)
Supplement: Supplementary file 1 [file Appendices.tex]

\section{Section title of first appendix}\label{secB}
